# Supplementary material for: Invalid Logic, Equivalent Gains: The Bizarreness of Reasoning in Language Model Prompting
Source: arXiv:2307.10573 source file (2023-07-23)
Supplement: Supplementary file 1 [file 05_appendix.tex]

\appendix
\onecolumn

\section{Choosing a Subset of BIG-Bench Hard}
\label{app:sec:bbh_subset}

Due to limited tokens and time, we were forced to focus on a subset of the BIG-Bench Hard (BBH) tasks. Specifically, we focused on the following tasks:

\begin{enumerate}
    \item Date Understanding: The question shall ask to decipher the actual date from a relative description to dates/events.
    \item Disambiguation QA: The subject of a verb is to be disambiguate between two or more nouns 
    \item Geometric Shapes: the shape of an object is to be determined by its SVG components
    \item Logical Deduction with Three Objects: The ordering of three objects is to be determined from the description
    \item Multi-step Arithmetic (Two): Arithmetic operations between 2 components, requiring multiple steps, is to be solved
    \item Reasoning about Colored Objects: Questions about a sequence of colored objects have to be answered
    \item Tracking Three Shuffled Objects: Colored objects are swapped amongst participants˜. The object has to be tracked to its final holder.
\end{enumerate}
